# Supplementary material for: Incremental Measurement of Structural Entropy for Dynamic Graphs
Source: arXiv:2207.12653 source file (2024-06-26)
Supplement: Supplementary file 1 [file 8-appendix.tex]

\section{Appendix} \label{sec:append}

\subsection{Dynamic Adjustment for One-Dimensional Encoding Trees}
In this part, we first give a formal description of the adjustment strategy for one-dimensional encoding trees.
Next, we derive the formula of the one-dimensional Local Difference.
Finally, we analyze the lower bound and the upper bound of the one-dimensional Local Difference.

\subsubsection{Strategy Description}
The dynamic adjustment strategy for the one-dimensional encoding tree is as follows.
\textit{When new graph nodes come, an equal number of leaf nodes are set as immediate successors of the root node. }
\textit{Each of new leaf nodes $\gamma$ has a single-node set label $T_\gamma = \{v\}$, where $v$ is one of the new graph nodes.}
Obviously, the updated one-dimensional encoding tree $\mathcal{T}'$ is also unique and optimal. 
So the updated one-dimensional entropy is always equal to the minimum structural entropy, i.e., $H^1(G')$.

\subsubsection{One-Dimensional Global Invariant and Local Difference}
Given a graph $G$ and its one-dimensional encoding tree $\mathcal{T}$,
the one-dimensional structural entropy of $G$ by $\mathcal{T}$ is defined as
\begin{equation}
    H^\mathcal{T}(G)=\sum_{v_i \in \mathcal{V}}-\frac{d_i}{2m}\log\frac{d_i}{2m}.
\label{1dSE}
\end{equation}
Since the one-dimensional encoding tree $\mathcal{T}$ has one unified form (like the one-dimensional encoding tree shown in Fig. \ref{intro2in1}(c)), it must be optimal. 
Therefore, $H^\mathcal{T}(G)$ is equal to the one-dimensional graph structural entropy $H^1(G)$.
Then, we give the definition of the one-dimensional Global Invariant and Local Difference based on Eq.~(\ref{1dSE}).
\begin{definition}[One-Dimensional Global Invariant and Local Difference]
Given an original graph $G$ and its one-dimensional encoding tree $\mathcal{T}$, the one-dimensional Global Invariant with incremental size $n$ is defined as
\begin{align}
H^\mathcal{T}_{GI}(G, n)=&\sum_{v_i \in \mathcal{V}}-\frac{d_i}{2(m+n)}\log\frac{d_i}{2(m+n)} \notag \\
=&-\frac{1}{2m+2n}(S_N+S_G),
\label{1dGI}
\end{align}
where

\begin{align}
S_N &= \sum_{v_i \in \mathcal{V}}d_i\log{d_i},\\
S_G &= -2m\log(2m+2n).
\end{align}
Given the updated graph $G'$, the updated one-dimensional encoding tree $\mathcal{T}'$, and the incremental size $n$, the one-dimensional Local Difference is defined as
\begin{equation}
\begin{aligned}
\Delta L_1 = H^{\mathcal{T}'}(G')-H^\mathcal{T}_{GI}(G, n).
\end{aligned}
\label{1dLD}
\end{equation}
\end{definition}

Suppose that after getting an incremental sequence $\xi$ with size $n$, the graph $G$ becomes $G'$ and its one-dimensional encoding tree $\mathcal{T}$ becomes $\mathcal{T}'$, the updated one-dimensional structural entropy can then be written as
\begin{equation}
\begin{aligned}
H^{\mathcal{T}'}(G')=&\sum_{v_i \in \mathcal{V}'}-\frac{d'_i}{2m+2n}\log\frac{d'_i}{2m+2n},
\end{aligned}
\label{1dSE-updated}
\end{equation}
where $\mathcal{V}'$ is the updated node set and $d'_i$ denotes the updated degree of $v_i$.
According to Eq.~(\ref{1dLD}), we get the one-dimensional Local Difference as
\begin{equation}
\begin{aligned}
\Delta L_1 =& H^{\mathcal{T}'}(G')-H^\mathcal{T}_{GI}(G,n)\\
=&-\frac{1}{2m+2n}(\Delta S_N + \Delta S_G),
\end{aligned}
\label{1dLD-unfold}
\end{equation}
where
\begin{align}
\Delta S_N &= \sum_{v_k \in \phi_\lambda}[(d_k+\delta(v_k))\log(d_k+\delta(v_k)) - d_k\log{d_k}],\\
\Delta S_G &= -2n\log(2m+2n).
\end{align}
$\delta(v_k)$ denotes the degree incremental $d'_k - d_k$, and $\phi_\lambda$ denotes the set of nodes that have changes in degree, i.e., $\phi_\lambda = \{v_k \in \mathcal{V}|\delta(v_k) \neq 0 \}$.

The properties of the two metrics are listed below.
On the one hand, the Global Invariant is an approximation of the updated structural entropy. 
Given an original graph $G$ and its encoding tree $\mathcal{T}$, the Global Invariant $H^\mathcal{T}_{GI}(G, n)$ is only dependent on the incremental size $n$.
Hence, the computational complexity of the Global Invariant is only $O(1)$ after recording the original graph's information.
On the other hand, the Local Difference represents the gap between the updated structural entropy and the Global Invariant, which is determined by a specific incremental sequence.
For an incremental sequence with size $n$, the computational complexity of the Local Difference is $O(n)$ both in the one-dimensional adjustment situation and our naive adjustment strategy for two-dimensional encoding trees (detailed in Section~\ref{sec:naive}).

\subsubsection{Boundedness Analysis} \label{sec:bound-1dLD}
We first analyze the maximum and minimum value of $\Delta S_N$ before we bound the Local Difference.
Let
\begin{equation}
s_N(d, x) = (d+x)\log(d+x) - d\log{d}.
\end{equation}
Since $s_N(d,n)$ is monotonically increasing with $d$, $\Delta S_N$ takes the maximum value when $n$ new incremental edges connect the two nodes with the largest degree.
Hence, we have
\begin{equation}
\Delta S_N \le 2s_N(d_{m},n),
\end{equation}
where $d_m$ denotes the maximum degree in $G$.
Since multiple edges are not allowed, the equality may hold if and only if $n = 1$.
When each of $n$ incremental edges connects a one-degree node and a new node, $\Delta S_N$ is minimized:
\begin{equation}
\Delta S_N \ge ns_N(1,0).
\end{equation}
Now we can get a lower bound of $\Delta L_1$ as
\begin{equation}
\begin{aligned}
\text{LB}(\Delta L_1)  = & -\frac{1}{2m+2n}(2s_N(d_m,n)+\Delta S_G)\\
= & \frac{1}{m+n}[d_m\log d_m-(d_m+n)\log{(d_m+n)} + n\log(2m+2n)].\\
\end{aligned}
\label{lb1}
\end{equation}
An upper bound of $\Delta L_1$ is
\begin{equation}
\begin{aligned}
\text{UB}(\Delta L_1) &= -\frac{1}{2m+2n}(ns_N(1,0)+\Delta S_G)\\
&= \frac{2n\log(2m+2n)+ n}{2m+2n}\\
&= \frac{n\log(m+n)+ \frac{3}{2}n}{m+n}.\\
\end{aligned}
\label{ub1}
\end{equation}

\subsubsection{Convergence Analysis}
In this section, we analyze the convergence of the one-dimensional Local Difference and its first-order absolute moment. 
We denote $g(m) = O(f(m))$ as $\lim_{m\rightarrow \infty}\frac{g(m)}{f(m)} = C$, where $C$ is a constant, to indicate that the $g(m)$ converges faster than or as fast as $f(m)$.

\begin{theorem}
Given the incremental size $n$, the one-dimensional Local Difference converges in order of $O(\frac{\log m}{m})$:
\begin{equation}
\begin{aligned}
\Delta L_{1} =& O(\frac{\log m}{m}).
\end{aligned}
\end{equation}
\label{conv-L1}
\end{theorem}
\textit{Proof.} 
According to Eq.~(\ref{lb1}) and Eq.~(\ref{ub1}), we have
\begin{align}
\text{LB}(\Delta L_1) = & \frac{d_m\log d_m-(d_m+n)\log{(d_m+n)}}{m+n} \notag + \frac{n}{m+n}\log(2m+2n) \notag\\
\ge & \frac{m\log m-(m+n)\log{(m+n)}}{m+n} \notag + \frac{n}{m+n}\log(2m+2n) \notag\\
= & \frac{1}{m+n}[\log (1-\frac{n}{m+n})^m +n] \notag\\
= & O(\frac{1}{m}),\\
\text{UB}(\Delta L_1) = & \frac{n\log(m+n)+ \frac{3}{2}n}{m+n} \notag\\
= & O(\frac{\log m}{m}).
\end{align}

Since
\begin{equation}
\begin{aligned}
 \text{LB}(\Delta L_1) \le \Delta L_1 \le \text{UB}(\Delta L_1),\\
\end{aligned}
\end{equation}
thus Theorem \ref{conv-L1} is proved. 
We can conclude that the gap between the updated one-dimensional structural entropy and the Global Invariant converges in order of $O(\frac{\log m}{m})$. 

\begin{definition}
Let $X$ be a random variable representing the incremental size $n$. We remind that $\mathbb{E}[X] = \overline n$.
\end{definition}
\begin{theorem}
The first-order absolute moment of the one-dimensional Local Difference converges in the order of $O(\frac{\log m}{m})$:
\begin{equation}
\begin{aligned}
\mathbb{E}[|\Delta L_{1}| ] = O(\frac{\log m}{m}).
\end{aligned}
\end{equation}
\label{first-order}
\end{theorem}
\textit{Proof.} 
By taking the expectation for the lower and upper bounds, we can obtain
\begin{align}
\mathbb{E}[|\text{LB}(\Delta L_1)|] = &  \mathbb{E}[|\frac{d_m\log d_m-(d_m+X)\log(d_m+X)}{m+X} +\frac{X\log(2m+2X)}{m+X}|] \notag\\
\le & \mathbb{E}[\frac{(m+X)\log{(m+X)}-m\log m}{m+X}] +\mathbb{E}[\frac{X\log(2m+2X)}{m+X}] \notag\\
\le & \frac{m\log m-(m+\overline n)\log{(m+\overline n)}}{m+\overline n} + \frac{\overline n\log(2m+2 \overline n)}{m+\overline n} \text{ (Jensen's inequality)} \notag\\
= & O(\frac{\log m}{m}),\\
\mathbb{E}[|\text{UB}(\Delta L_1)|] = &  \mathbb{E}[\frac{ X\log(m+X) + \frac{3}{2}X}{m+X}] \notag\\
\le & \frac{ \overline n\log(m+ \overline n) + \frac{3}{2}\overline n}{m+\overline n} \text{ (Jensen's inequality)} \notag\\
= & O(\frac{\log m}{m}).
\end{align}
Since
\begin{equation}
\begin{aligned}
0 \le \mathbb{E}[|\Delta L_1|] \le \max\{ \mathbb{E}[|\text{LB}(\Delta L_1)|], \mathbb{E}[|\text{UB}(\Delta L_1)|]\},
\end{aligned}
\end{equation}
theorem \ref{first-order} is proved.
We can conclude that the expectation of the absolute value (i.e., the first-order absolute moment) of one-dimensional Local Difference converges in order of $O(\frac{\log m}{m})$.
